# Supplementary material for: Neutrino flux sensitivity to the next galactic core-collapse supernova in COSINUS
Source: arXiv:2409.09109 source file (2025-02-06)
Supplement: Supplementary file 1 [file NeutrinoElectronScattering_Appendix.tex]

\section{Electron-Neutrino Scattering}\label{App:Electron_Neutrino_Scattering}

As discussed in Sec.~\ref{subsec:Water_Tank_Interactions} neutrinos can scatter off the electrons present in the water tank. Traditionally, this interaction can provide some directionality with regard to the location of the supernova. This process is sensitive to all flavors of neutrinos and the  differential recoil rate is described as
\begin{equation}\label{Eqn:Diff_Recoil_ES}
    \frac{dR}{dE_e} = {N_e}\int_{E^{\text{min}}_\nu} \Phi^d(E_{\nu}) \frac{d\sigma_t}{dE_e} dE_{\nu},
\end{equation}
where $N_e$ is the number of target electrons and $\Phi^d (E_\nu)$ is the neutrino flux defined by Eqn.~\ref{Eqn:Neutrino_Flux_1}. Based of conservation of momentum, the minimum neutrino energy to generate a electron recoil of energy $E_e$ can be written as
\begin{equation}\label{Eqn:Enu_min_ES}
    E_\nu^{\text{min}} = \frac{E_e}{2}\left(1+\sqrt{1+\frac{2 m_e}{E_e}}\right)
\end{equation}
where $m_e$ is the mass of the electron. From~\cite{giunti2007fundamentals} the differential cross-section can be written as  

\begin{equation}\label{Eqn:Diff_Cross_Section_ES}
\frac{d\sigma}{dE_e} = \frac{2 G_f^2 m_e}{\pi} \left[g_1^2+g_2^2(1-\frac{E_e}{E_\nu})^2-g_1g_2 \frac{m_e E_e}{E_\nu^2}\right], 
\end{equation}
with the coefficients $g_1$ and $g_2$ being different for each flavor of neutrino, see Table~\ref{tab:Diff_Cross_Sec_Constants}.

\begin{table}[ht]
    \centering
    \begin{tabular}{c|cccc}
    \hline
    & $\nu_e$ & $\bar{\nu}_e$  & $\nu_x$ & $\bar{\nu}_x$ \\\hline
    $g_1$  & $\frac{1}{2} +$ sin$^2\theta_w$ & sin$^2\theta_w$  & -$\frac{1}{2} +$ sin$^2\theta_w$ & sin$^2\theta_w$  \\
    $g_2$  & sin$^2\theta_w$ & $\frac{1}{2} +$ sin$^2\theta_w$ & sin$^2\theta_w$ & -$\frac{1}{2} +$ sin$^2\theta_w$\\
    
    \end{tabular}
    \caption{Neutrino flavor dependent differential cross-section coefficients. }
    \label{tab:Diff_Cross_Sec_Constants}
\end{table}

For a supernova at 10~kpc the differential recoil spectrum is shown in Fig.~\ref{Fig:ES_Recoil_Spectrum.pdf}. Both the normal and inverse ordering scenario are shown, as well the efficiency from Fig.~\ref{Fig: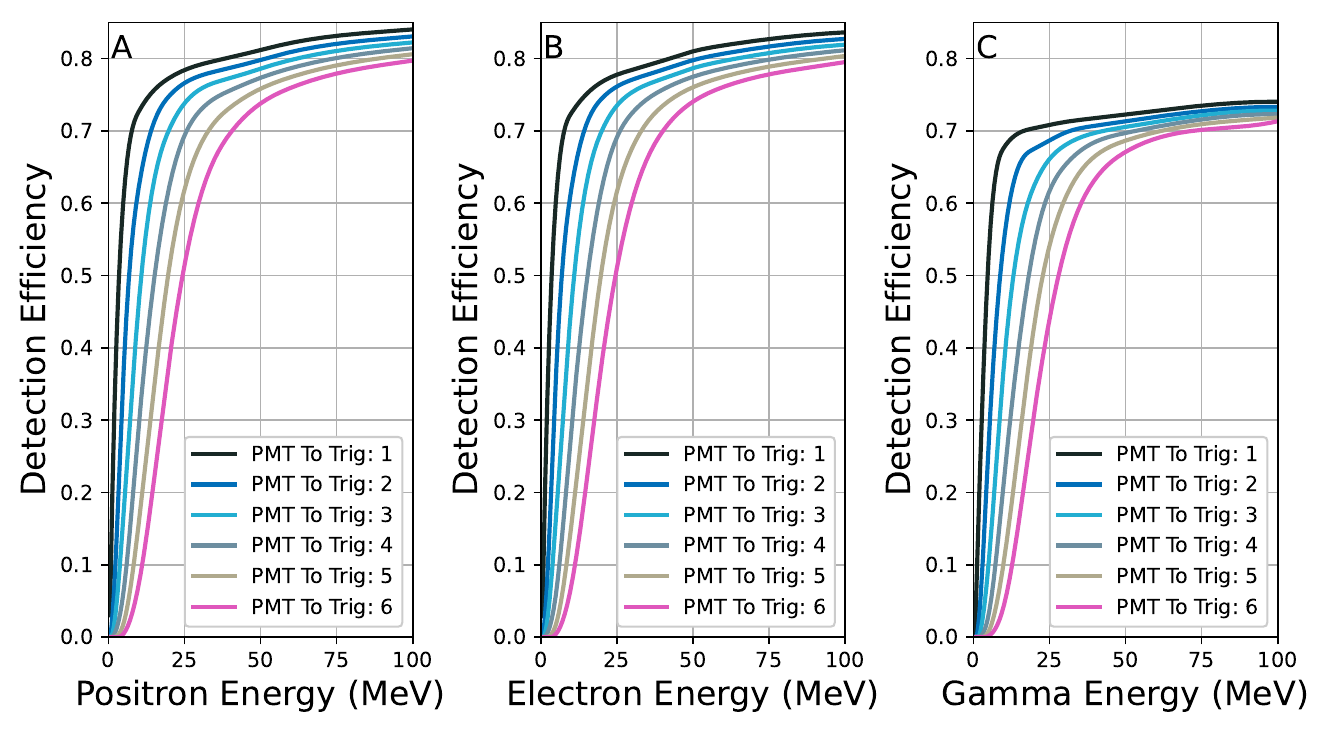} is folded in. By integrating the spectra and multiplying by the water tank mass the total number of electron scattering events can be calculated. Table~\ref{tab:10kpc_ES_Events} shows the number of events for a supernova at 10~kpc. Repeating the above process for different supernovae distances a profile of the total number of electron scattering events can be built, shown in Fig.~\ref{Fig:Electron_Scattering_Events_vs_Distance}. As shown, electron scattering will contribute only a small percentage of the total number of neutrino interactions and will only be relevent for very close supernovae.
\begin{figure*}[ht]
\begin{subfigure}[t]{0.50\textwidth}
\includegraphics[width=\textwidth]{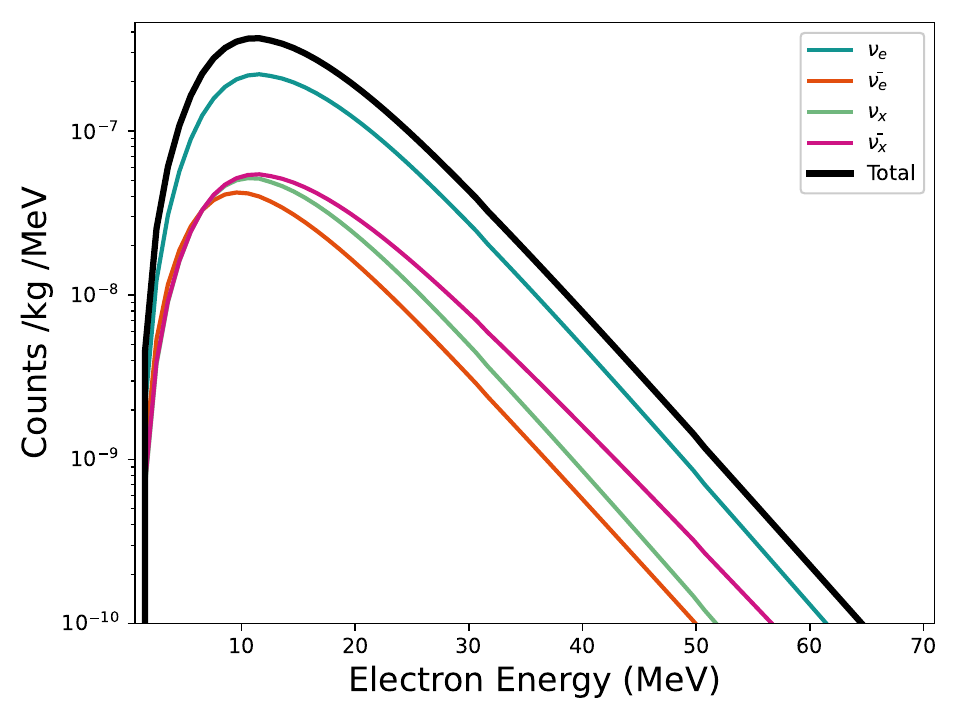} 
\caption{$27M_\odot$}
\end{subfigure}
\begin{subfigure}[t]{0.50\textwidth}
\includegraphics[width=\textwidth]{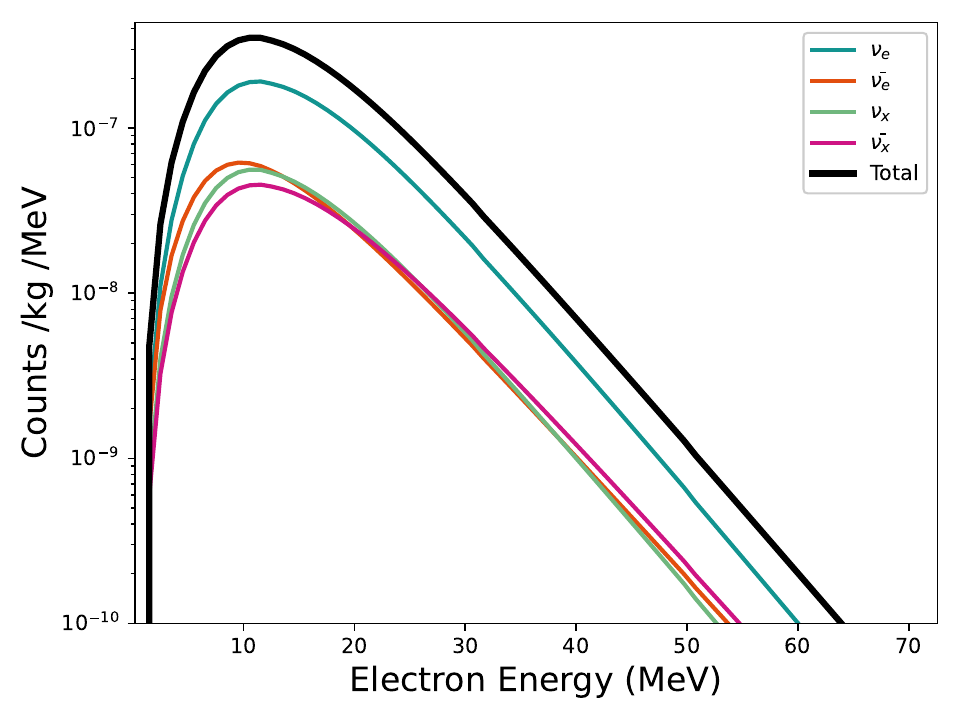}
\caption{$27M_\odot$}
\end{subfigure}
\begin{subfigure}[t]{0.5\textwidth}
\includegraphics[width=\textwidth]{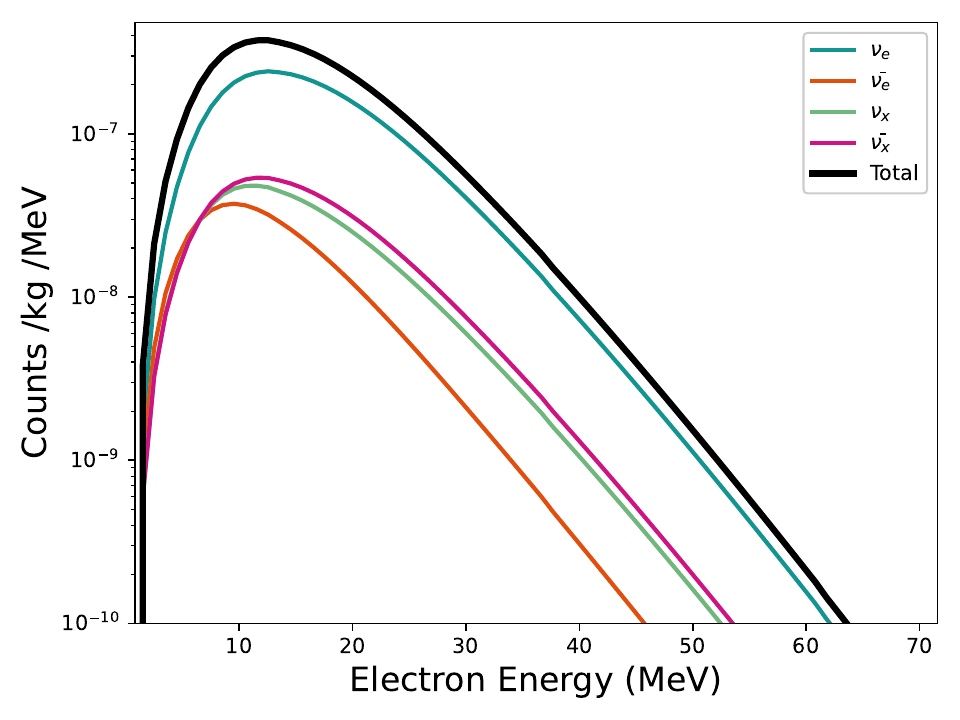} 
\caption{1987A-like}
\end{subfigure}
\begin{subfigure}[t]{0.5\textwidth}
\includegraphics[width=\textwidth]{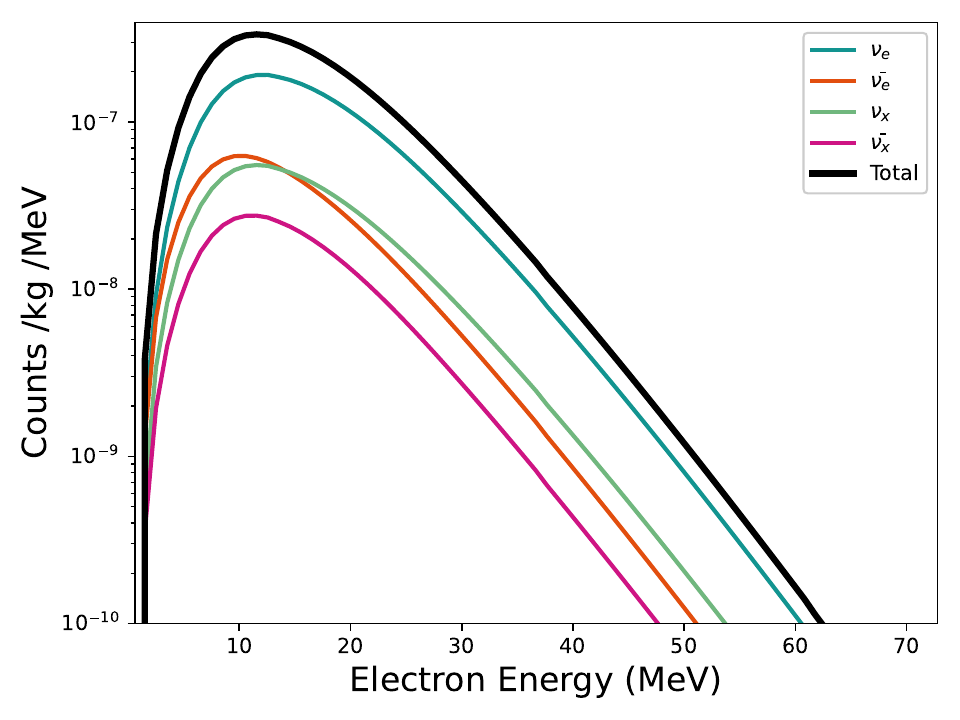}
\caption{1987A-like}
\end{subfigure}
\caption{Electron recoil energy spectrum for neutrino scattering in water from a 10~kpc away supernova for both the normal ordering (a)(c) and inverse ordering (b)(d) scenario. The efficiency from Fig.~\ref{Fig:Water_Tank_Detection_Efficiency.pdf} is used, specifically the scenario where 4 PMTs are required to trigger for a single event.  Upper graphs (a)(b) correspond to $27M_\odot$ data, and lower graphs (c)(d) correspond to 1987A-like data.}\label{Fig:ES_Recoil_Spectrum.pdf}
\end{figure*}

\begin{table}[ht]
    \centering
    \begin{tabular}{c|c|c|cccc|c}
    \hline
    Flux & Ordering & PMT Threshold& $\nu_e$ & $\bar{\nu}_e$  & $\nu_x$ & $\bar{\nu}_x$ & Total\\\hline
   1987A & NO & 4  & 1.64 & 0.17 & 0.31 & 0.34 & 2.46 \\
   1987A & IO & 4  & 1.30 & 0.30 & 0.36 & 0.17 & 2.13 \\
   1987A & NO & 6  & 0.92 & 0.075 & 0.16 & 0.18 & 1.34 \\
   1987A & IO & 6  & 0.70 & 0.14 & 0.19 & 0.08 & 1.11 \\
   $27M_\odot$ & NO & 4  & 1.45 & 0.20 & 0.32 & 0.35 & 2.32 \\
   $27M_\odot$ & IO & 4  & 1.24 & 0.30 & 0.35 & 0.29 & 2.18 \\
   $27M_\odot$ & NO & 6  & 0.75 & 0.09 & 0.16  & 0.18 & 1.18  \\
   $27M_\odot$ & IO & 6  & 0.63 & 0.14 & 0.18 & 0.15 & 1.10 \\
    
    \end{tabular}
    \caption{Number of electron scattering events for the different neutrino flavors for a supernova at 10~kpc.}
    \label{tab:10kpc_ES_Events}
\end{table}

\begin{figure*}[ht]
\begin{subfigure}[t]{0.50\textwidth}
\includegraphics[width=\textwidth]{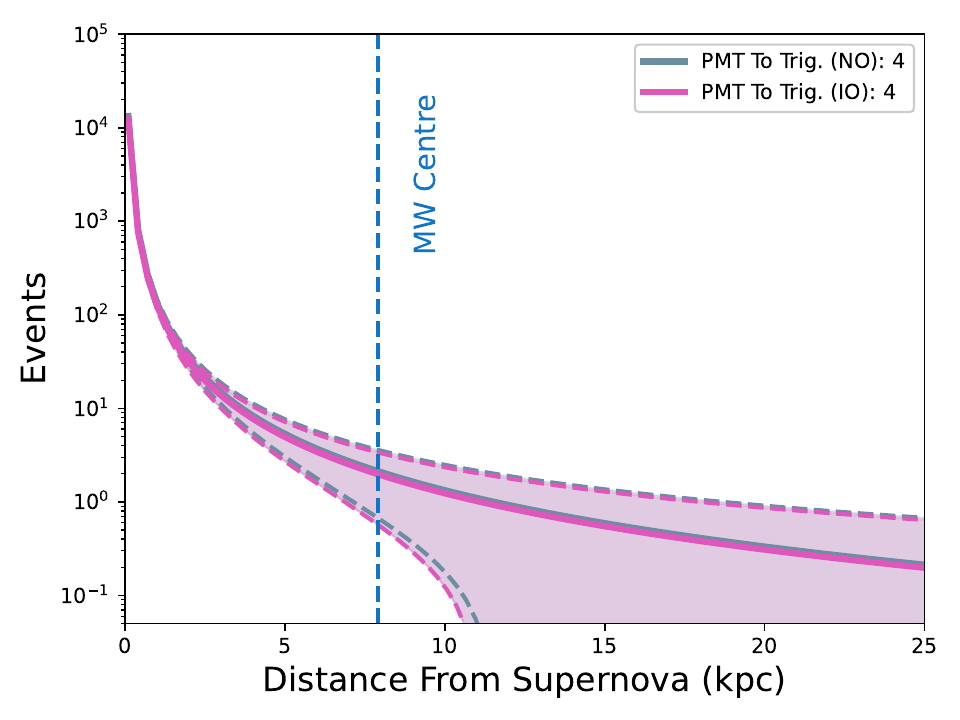} 
\caption{$27M_\odot$}
\end{subfigure}
\begin{subfigure}[t]{0.50\textwidth}
\includegraphics[width=\textwidth]{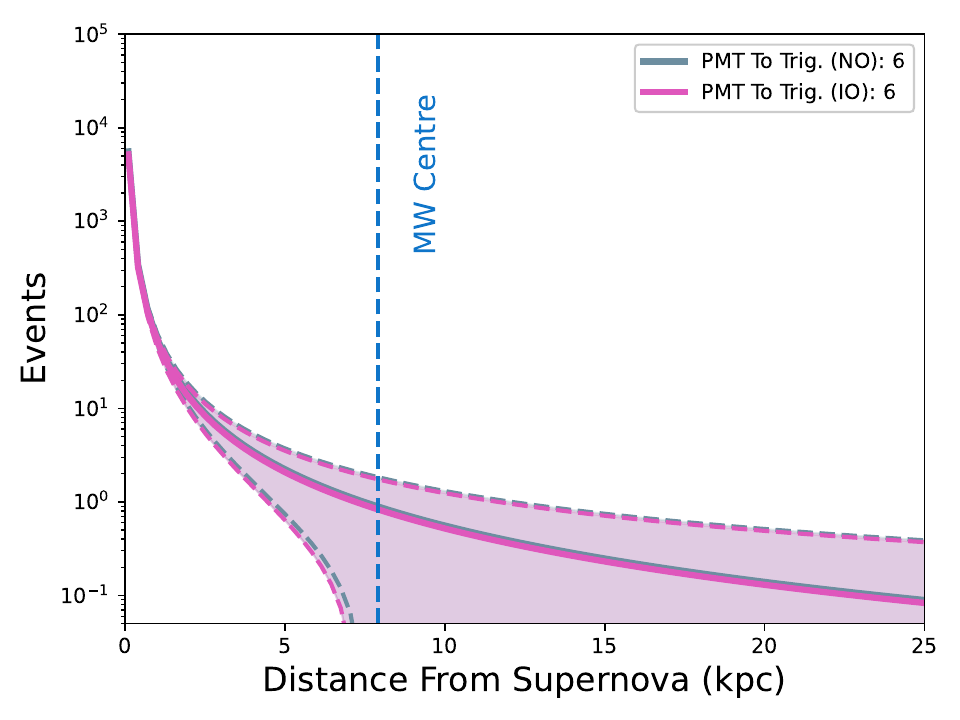}
\caption{$27M_\odot$}
\end{subfigure}
\begin{subfigure}[t]{0.5\textwidth}
\includegraphics[width=\textwidth]{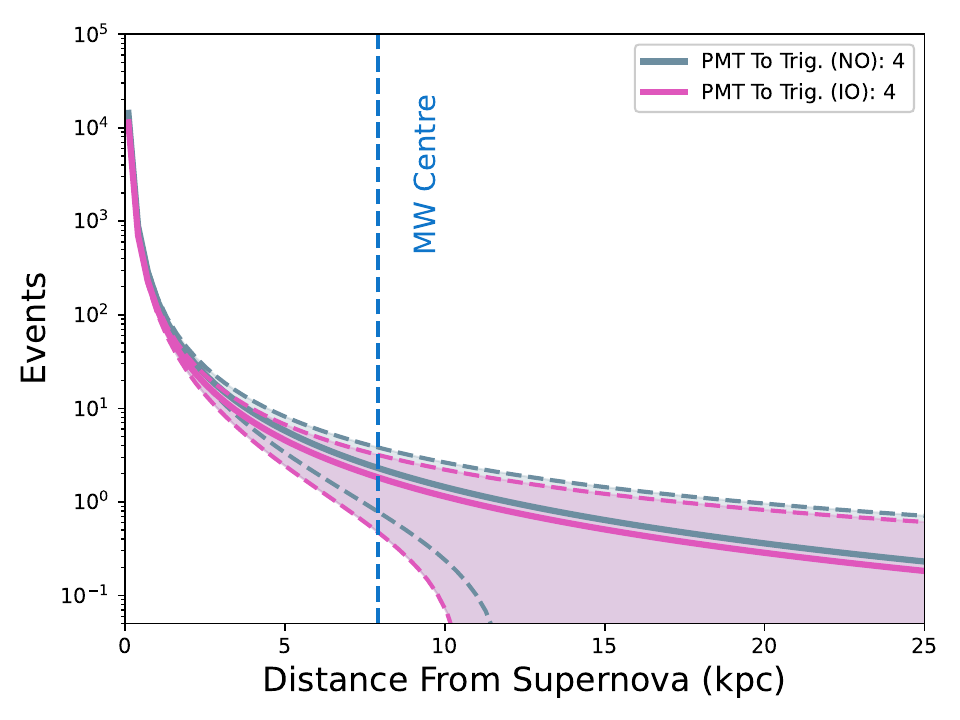} 
\caption{1987A-like}
\end{subfigure}
\begin{subfigure}[t]{0.5\textwidth}
\includegraphics[width=\textwidth]{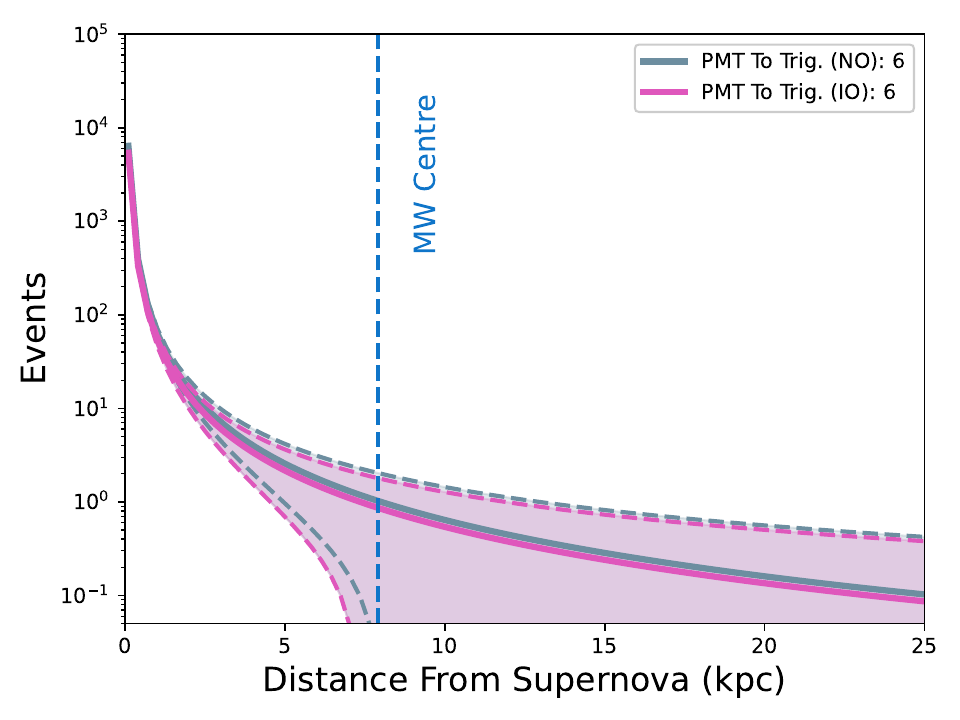}
\caption{1987A-like}
\end{subfigure}
\caption{Expected number of electron scattering events in the COSINUS water Cherenkov detector as a function of the supernova distances. Both the normal and inverted ordering scenario were considered for a 4 (a)(c) and 6 (b)(d) PMT trigger threshold. Upper graphs (a)(b) correspond to $27M_\odot$ data, and lower graphs (c)(d) correspond to 1987A-like data.}\label{Fig:Electron_Scattering_Events_vs_Distance}
\end{figure*}
